# Supplementary material for: Recall Traces: Backtracking Models for Efficient Reinforcement Learning
Source: arXiv:1804.00379 source file (2019-01-28)
Supplement: Supplementary file 1 [file supplementary.tex]

%%%%%%%% ICML 2018 EXAMPLE LATEX SUBMISSION FILE %%%%%%%%%%%%%%%%%

\documentclass{article}

% Recommended, but optional, packages for figures and better typesetting:
\usepackage{microtype}
\usepackage{graphicx}
\usepackage{booktabs} % for professional tables
\usepackage{color}
\usepackage{subfig}
\usepackage{amsmath,amssymb}

% hyperref makes hyperlinks in the resulting PDF.
% If your build breaks (sometimes temporarily if a hyperlink spans a page)
% please comment out the following usepackage line and replace
% \usepackage{icml2018} with \usepackage[nohyperref]{icml2018} above.
\usepackage{hyperref}
\usepackage[title]{appendix}

% Attempt to make hyperref and algorithmic work together better:

% Use the following line for the initial blind version submitted for review:
\usepackage{icml2018}

% Added commands

% If accepted, instead use the following line for the camera-ready submission:
%\usepackage[accepted]{icml2018}

% The \icmltitle you define below is probably too long as a header.
% Therefore, a short form for the running title is supplied here:
\icmltitlerunning{Recall Traces: Backtracking Models for Efficient Reinforcement Learning}

\begin{document}

%\twocolumn[
%\icmltitle{Recall Traces: Backtracking Models for Efficient Reinforcement Learning}

\input{appendix}

%\clearpage
\bibliography{bibliography}
\bibliographystyle{icml2018}

\clearpage
\appendix

\end{document}
